# Supplementary material for: Enhanced orientational ordering induced by active yet isotropic bath
Source: arXiv:1909.12014 ancillary file (2019-09-27)
Supplement: Supplementary file 1 [file act_ord_supp2.pdf]

# Enhanced orientational ordering induced by active yet isotropic bath: Supplementary material

Ananyo Maitra[1,*] and Raphael Voituriez[1,2]

[1] *Sorbonne Université and CNRS, Laboratoire Jean Perrin, F-75005, Paris, France*

[2] *Sorbonne Université and CNRS, Laboratoire de Physique Théorique de la Matière Condensée, F-75005, Paris, France*

In this supplement, we detail the calculations leading to the results presented in the main text. In Sec. I, we present the detailed calculations for the $\phi^4$ theory, in Sec. II, for the polar model, in Sec. III for the apolar model, and finally in Sec. IV we demonstrate that the effective $\phi^4$ free energy obtained within our theory of the $\phi^4$ model coupled to an autonomous active field reduces to the one obtained for a $\phi^4$ theory with a exponentially-correlated coloured noise driving within a unified coloured noise approximation [1], to $\mathcal{O}(\tau_\phi)$, in the $D = 0$ limit.

## I. DETAILED CALCULATION FOR THE $\phi^4$ MODEL

We start with a $\phi^4$ model with a nonequilibrium coupling to a field $\xi_c$ whose dynamics is autonomous and unaffected by $\phi$

$$\partial_t \phi(\mathbf{x}, t) = -\frac{\delta F_\phi}{\delta \phi(\mathbf{x})} + c\xi_c(\mathbf{x}, t) + \xi_\phi(\mathbf{x}, t), \tag{S1}$$

where

$$F_\phi = \int d\mathbf{x} \left[\frac{\alpha}{2}\phi^2 + \frac{\beta}{4}\phi^4 + \frac{K}{2}(\nabla\phi)^2\right], \tag{S2}$$

and

$$\tau_\phi \partial_t \xi_c = -\xi_c + \zeta \tag{S3}$$

where $\langle \zeta(\mathbf{x}, t)\zeta(\mathbf{x}', t')\rangle = 2\tilde{D}_\phi \delta(\mathbf{x} - \mathbf{x}')\delta(t - t')$ and $\langle \xi_\phi(\mathbf{x}, t)\xi_\phi(\mathbf{x}', t')\rangle = 2D\delta(\mathbf{x} - \mathbf{x}')\delta(t - t')$. $\xi_c$ is now interpreted as an autonomously relaxing field that actively couples with $\phi$ and we have introduced a coupling constant $c$ with $c \to 0$ implying a detailed balance obeying dynamics. The Fokker-Planck equation for $\Pi(\phi, \xi_c)$ is

$$\partial_t \Pi = \int d\mathbf{x} \frac{\delta}{\delta\phi}[-c\xi_c \Pi] + D\frac{\delta^2 \Pi}{\delta\phi^2} + \frac{\delta}{\delta\phi}\left(\frac{\delta F_\phi}{\delta\phi}\Pi\right) + \frac{1}{\tau_\phi}\left[\frac{\delta}{\delta\xi_c}\left(\xi_c \Pi + \frac{\tilde{D}_\phi}{\tau_\phi}\frac{\delta\Pi}{\delta\xi_c}\right)\right]. \tag{S4}$$

We would like to calculate the distribution function for $\phi$, marginalised with respect to $\xi_c$, i.e., $\int \mathcal{D}\xi_c \Pi$ to first order in $\tau_\phi$. For this, we define the moments $R_k[\phi] = \int \mathcal{D}\xi_c \xi_c^k \Pi$. The equations of the moments are

$$\partial_t R_0 = \int d\mathbf{x} \left[-c\frac{\delta R_1}{\delta\phi(\mathbf{x})} + D\frac{\delta^2 R_0}{\delta\phi(\mathbf{x})\delta\phi(\mathbf{x})} + \frac{\delta}{\delta\phi(\mathbf{x})}\left(\frac{\delta F_\phi}{\delta\phi(\mathbf{x})}R_0\right)\right] \tag{S5}$$

$$\partial_t R_1 = \int d\mathbf{x} \left[-c\frac{\delta R_2}{\delta\phi(\mathbf{x})} + D\frac{\delta^2 R_1}{\delta\phi(\mathbf{x})\delta\phi(\mathbf{x})} + \frac{\delta}{\delta\phi(\mathbf{x})}\left(\frac{\delta F_\phi}{\delta\phi(\mathbf{x})}R_1\right) - \frac{R_1}{\tau_\phi}\right] \tag{S6}$$

$$\partial_t R_2 = \int d\mathbf{x} \left[-c\frac{\delta R_3}{\delta\phi(\mathbf{x})} + D\frac{\delta^2 R_2}{\delta\phi(\mathbf{x})\delta\phi(\mathbf{x})} + \frac{\delta}{\delta\phi(\mathbf{x})}\left(\frac{\delta F_\phi}{\delta\phi(\mathbf{x})}R_2\right) - \frac{2R_2}{\tau_\phi} + \frac{2\tilde{D}_\phi R_0}{\tau_\phi^2}\right] \tag{S7}$$

$$\partial_t R_3 = \int d\mathbf{x} \left[-c\frac{\delta R_4}{\delta\phi(\mathbf{x})} + D\frac{\delta^2 R_3}{\delta\phi(\mathbf{x})\delta\phi(\mathbf{x})} + \frac{\delta}{\delta\phi(\mathbf{x})}\left(\frac{\delta F_\phi}{\delta\phi(\mathbf{x})}R_3\right) - \frac{3R_3}{\tau_\phi} + \frac{6\tilde{D}_\phi R_1}{\tau_\phi^2}\right] \tag{S8}$$

The marginalised steady-state distribution $R_0$ is obtained in the $\tau_\phi \to 0$ limit by using (S7) to express $R_2$ in terms of $R_0$, $R_2 = \tilde{D}_\phi R_0/\tau_\phi$, which, matching the lowest order in $\tau_\phi$ terms in (S6) implies

$$R_1 = -c\tilde{D}_\phi \frac{\delta R_0}{\delta\phi(\mathbf{x})} \tag{S9}$$

Inserting this in (S5) leads to the distribution

$$R_0 \propto e^{F_\phi/(D+c^2\tilde{D}_\phi)} \tag{S10}$$

i.e., at zeroth order in $\tau_\phi$, the $\xi_c$ field leads to an additional white noise of strength $2c^2\tilde{D}_\phi$ in the dynamics of $\phi$ with the total noise-strength being $\tilde{D} = D + c^2\tilde{D}_\phi$. To calculate $R_0$ to first order in $\tau_\phi$, we need to start with (S8) to obtain $R_3 = 2\tilde{D}_\phi R_1/\tau_\phi$ which, from (S7), yields

$$R_2 = \frac{\tilde{D}_\phi}{\tau_\phi} R_0 - c\tilde{D}_\phi \frac{\delta R_1}{\delta\phi} \tag{S11}$$

Using this in (S6) at steady-state yields

$$R_1 = -c\tilde{D}_\phi \frac{\delta R_0}{\delta\phi(\mathbf{x})} + \tau_\phi \left[\tilde{D}\frac{\delta^2 R_1}{\delta\phi(\mathbf{x})\delta\phi(\mathbf{x})} + \frac{\delta}{\delta\phi(\mathbf{x})}\left(\frac{\delta F_\phi}{\delta\phi(\mathbf{x})} R_1\right)\right]. \tag{S12}$$

Using this in (S5) we obtain

$$\tilde{D}\frac{\delta^2 R_0}{\delta\phi(\mathbf{x})\delta\phi(\mathbf{x})} + \frac{\delta}{\delta\phi(\mathbf{x})}\left(\frac{\delta F_\phi}{\delta\phi(\mathbf{x})} R_0\right) = c\tau_\phi \frac{\delta}{\delta\phi}\left[\tilde{D}\frac{\delta^2 R_1}{\delta\phi(\mathbf{x})\delta\phi(\mathbf{x})} + \frac{\delta}{\delta\phi(\mathbf{x})}\left(\frac{\delta F_\phi}{\delta\phi(\mathbf{x})} R_1\right)\right]. \tag{S13}$$

We now expand $R_0 = R_0^0 + \tau_\phi R_0^1$, $R_1 = R_1^0 + \tau_\phi R_1^1$ with $R_0^0 = e^{-F_\phi/\tilde{D}}$ and

$$R_1^0 = \frac{c\tilde{D}_\phi}{\tilde{D}} \frac{\delta F_\phi}{\delta\phi} R_0^0 \tag{S14}$$

to obtain

$$\tilde{D}\frac{\delta R_0^1}{\delta\phi(\mathbf{x})} + \frac{\delta F_\phi}{\delta\phi(\mathbf{x})} R_0^1 = c\left[\tilde{D}\frac{\delta^2 R_1^0}{\delta\phi(\mathbf{x})\delta\phi(\mathbf{x})} + \frac{\delta}{\delta\phi(\mathbf{x})}\left(\frac{\delta F_\phi}{\delta\phi(\mathbf{x})} R_1^0\right)\right]. \tag{S15}$$

This yields

$$\frac{\delta}{\delta\phi}\left[e^{F_\phi/\tilde{D}} R_0^1\right] = \frac{c^2\tilde{D}_\phi}{\tilde{D}} \frac{\delta}{\delta\phi}\left[\frac{\delta^2 F_\phi}{\delta\phi^2} - \frac{1}{2\tilde{D}}\left(\frac{\delta F_\phi}{\delta\phi}\right)^2\right] \tag{S16}$$

Thus,

$$R_0 = R_0^0 + \tau_\phi R_0^1 = e^{-F_\phi/\tilde{D}}\left[1 - \frac{c^2\tilde{D}_\phi\tau_\phi}{\tilde{D}^2}\left\{\frac{1}{2}\left(\frac{\delta F_\phi}{\delta\phi}\right)^2 - \tilde{D}\frac{\delta^2 F_\phi}{\delta\phi^2}\right\}\right] \overset{\mathcal{O}(\tau_\phi)}{=} e^{-\frac{1}{\tilde{D}}\left[F_\phi + \frac{c^2\tilde{D}_\phi\tau_\phi}{\tilde{D}}\left\{\frac{1}{2}\left(\frac{\delta F_\phi}{\delta\phi}\right)^2 - \tilde{D}\frac{\delta^2 F_\phi}{\delta\phi^2}\right\}\right]} = e^{-\tilde{F}_\phi/\tilde{D}} \tag{S17}$$

where we retain only the terms explicitly containing $\phi$ for the expression within the curly brackets (every term not dependent on $\phi$ would be eliminated by the functional derivative with respect to $\phi$ on the R.H.S of (S16)). This yields

$$\tilde{F}_\phi = \frac{1}{2}\int d\mathbf{x}\Big[\{\alpha + \frac{\tau_\phi c^2\tilde{D}_\phi}{\tilde{D}}(\alpha^2 - 6\tilde{D}\beta)\}\phi^2 + \beta\left(\frac{\tilde{D} + 4c^2\tau_\phi\alpha\tilde{D}_\phi}{2\tilde{D}}\right)\phi^4 + K\left(1 + 2\frac{\tau_\phi c^2\tilde{D}_\phi}{\tilde{D}}\alpha\right)(\nabla\phi)^2$$
$$+ \frac{\tau_\phi c^2\tilde{D}_\phi}{\tilde{D}}\beta^2\phi^6 + \frac{\tau_\phi c^2\tilde{D}_\phi}{\tilde{D}}K(\nabla^2\phi)^2 + 6\frac{\tau_\phi c^2\tilde{D}_\phi}{\tilde{D}}\beta K\phi^2(\nabla\phi)^2\Big] \tag{S18}$$

where we have used the expression for $F_\phi$ from (S2) explicitly.

In the main text, using (S18), we show that the effect of the coupling to the active field with the correlation time $\tau_\phi$, via $c$ shifts the critical point upwards, both in the mean-field theory and within a self-consistent approximation. Here, we argue that this conclusion is valid more generally. Generally, the shift from the mean-field critical point due to fluctuations has to be a function of the nonlinear parameter (it is not a universal quantity and therefore, must depend on the parameters of the system). We can therefore assume that the condition for criticality, after all fluctuation corrections are taken into account, is

$$0 = \bar{\alpha} + g\left(\frac{\tilde{D}\bar{\beta}}{\bar{K}}\right) \tag{S19}$$

where $\bar{\alpha}$, $\bar{\beta}$ and $\bar{K}$ are the coefficients of the terms $\phi^2/2$, $\phi^4/4$ and $(\nabla\phi)^2/2$ respectively, in the free energy $\tilde{F}_\phi$ and the function $g(u)$ denotes the correction to the bare mass at criticality due to the nonlinearity. Note that since the function $g(u)$ has to be a characteristic of the $\phi^4$ theory, the condition for criticality for a free-energy with $\tau_\phi = 0$ (but $c \neq 0$) must be

$$0 = \alpha + g\left(\frac{\tilde{D}\beta}{K}\right). \tag{S20}$$

Since $\bar{\beta} = \beta[1 + 4c^2\tau_\phi\alpha(\tilde{D}_\phi/\tilde{D})]$ and $\bar{K} = K[1 + 2c^2\tau_\phi\alpha(\tilde{D}_\phi/\tilde{D})]$, to first order in $\tau_\phi$,

$$\frac{\bar{\beta}}{\bar{K}} = \frac{\beta}{K}[1 + 2c^2\tau_\phi\alpha(\tilde{D}_\phi/\tilde{D})]. \tag{S21}$$

We can now Taylor expand $g(\tilde{D}\bar{\beta}/\bar{K})$ around $g(\tilde{D}\beta/K)$ to first order in $\tau_\phi$:

$$g\left(\frac{\tilde{D}\bar{\beta}}{\bar{K}}\right) = g\left(\frac{\tilde{D}\beta}{K}\right) + 2c^2\tau_\phi\alpha\tilde{D}_\phi\frac{\beta}{K}g'(u)|_{u=\tilde{D}\beta/K}, \tag{S22}$$

where the prime denotes differentiation. Define the value of $\alpha$ at criticality, $\alpha^c = \alpha_0 + \tau_\phi\alpha_1$. Obviously, $\alpha_0 = -g(\tilde{D}\beta/K)$. Now,

$$\bar{\alpha} = \alpha + \tau_\phi c^2\frac{\tilde{D}_\phi}{\tilde{D}}(\alpha^2 - 6\tilde{D}\beta). \tag{S23}$$

Therefore, the equation for $\alpha_1$ is

$$\alpha_1 = 6c^2\tilde{D}_\phi\beta + c^2\frac{\tilde{D}_\phi}{\tilde{D}}\left[2\frac{\tilde{D}\beta}{K}g\left(\frac{\tilde{D}\beta}{K}\right)g'\left(\frac{\tilde{D}\beta}{K}\right) - g^2\left(\frac{\tilde{D}\beta}{K}\right)\right]. \tag{S24}$$

The condition for the term in the square brackets to be positive is simply that $g(u) > 0$ for all $u$ (which is obviously satisfied since otherwise it would mean that fluctuations would shif the critical point upwards) and $g'(u) > g(u)/2$ which implies that $g(u)$ grows faster than $u^{1/2}$. If $g(u)$ grows slower than $u^{1/2}$ (or even decays with $u$), the term in the square brackets, which scales as $g^2(u)$, grows slower than $\tilde{D}$ and therefore, slower than $\tilde{D}_\phi$ as $\tilde{D}_\phi$ is increased. Therefore, $\alpha_1$ still increases as $\tilde{D}_\phi$ is increased since the first term increases as $\tilde{D}_\phi$. Thus, at large enough active noise strengths, the $\tau_\phi$ dependent correction to the critical point always increases with the noise strength.

This compares a model with $c \neq 0$ but $\tau_\phi = 0$ to one with $c \neq 0$ and $\tau_\phi \neq 0$. For a model with $c = 0$ instead, at criticality, $\alpha^0 = -g(D\beta/K)$. Therefore,

$$\alpha^c - \alpha^0 = -g\left(\frac{\tilde{D}\beta}{K}\right) + g\left(\frac{D\beta}{K}\right) + 6\tau_\phi c^2\tilde{D}_\phi\beta + \tau_\phi c^2\frac{\tilde{D}_\phi}{\tilde{D}}\left[2\frac{\tilde{D}\beta}{K}g\left(\frac{\tilde{D}\beta}{K}\right)g'\left(\frac{\tilde{D}\beta}{K}\right) - g^2\left(\frac{\tilde{D}\beta}{K}\right)\right]. \tag{S25}$$

For $g(u)$ growing faster than $u^{1/2}$, the term in the square bracket is positive, and grows faster as a function of $\tilde{D}_\phi$ than the combination of the first two terms, leading to an active upward shift of the critical point. If $g(u)$ grows slower than $u^{1/2}$, the term in the square brackets is negative, but $6\tau_\phi c^2\tilde{D}_\phi\beta$ grows faster than all other terms as $\tilde{D}_\phi$ is increased, again leading to an upward shift of the critical point.

More qualitatively, $\bar{\alpha}\phi^2$ is relevant in any dimension, i.e., its value has to be tuned (to 0 for $d > 4$ and to $-\epsilon/6$, $\epsilon = 4 - d$ for $d < 4$) to reach criticality in any dimension. Our calculation shows that this parameter can be tuned to criticality by increasing the active noise-strength.

## II. DETAILED CALCULATION FOR THE POLAR MODEL

We now consider the dynamics of a population of polar rods in a bath of isotropic but active beads on a substrate. The polarisation of the passive rods responds to the local velocity field produced by the beads and other rods, and not only its gradient. Therefore, a simple model of the dynamics of the polar order parameter and the overdamped centre-of-mass velocity is

$$D_t\mathbf{p} = \Lambda\mathbf{v} - \Gamma_p\frac{\delta F_p}{\delta\mathbf{p}} + \sqrt{2D\Gamma_p}\boldsymbol{\xi}_p \tag{S26}$$

$$\gamma \mathbf{v} = \upsilon \mathbf{m} - \Lambda \frac{\delta F_p}{\delta \mathbf{p}} + \sqrt{2D\gamma}\boldsymbol{\xi}_v \tag{S27}$$

where $F_p = \int d\mathbf{x} f_p$

$$f_p = \frac{\alpha}{2}\mathbf{p}\cdot\mathbf{p} + \frac{\beta}{4}(\mathbf{p}\cdot\mathbf{p})^2, \tag{S28}$$

$\boldsymbol{\xi}_p$ and $\boldsymbol{\xi}_v$ are unit-variance Gaussian white noises and $\gamma$ is the friction coefficient. The term with coefficient $\Lambda$ is an *equilibrium* coupling to the polarisation field required by Onsager symmetry and $\mathbf{m}$ is the polarisation field of AOUPs which leads to an active force in (S27). We assume that the number density of the AOUPs is not conserved (i.e., they can move in and out of the system) to eliminate the effect of long-range interaction that such a conservation law could mediate [2]. We further do not explicitly consider the dynamics of density of the polar rods $\rho$ since the coupling between $\rho$ and $\mathbf{p}$ (due to a free energy term $\rho\nabla\cdot\mathbf{p}$) can not change the mean-field critical point. The polarisation field of AOUPs is taken to relax autonomously

$$\tau_p \partial_t \mathbf{m} = -\mathbf{m} + \sqrt{2D_m}\boldsymbol{\xi}_m. \tag{S29}$$

Eliminating $\mathbf{v}$ and defining $\nu = \Lambda\upsilon/\gamma$ and $\tilde{\Gamma}_p = \Gamma_p + \Lambda^2/\gamma$, we obtain

$$\partial_t \mathbf{p} = -\tilde{\Gamma}_p \mathbf{h} + \nu\mathbf{m} + \sqrt{2D\tilde{\Gamma}_p}\boldsymbol{\xi}_p, \tag{S30}$$

where $\mathbf{h} = \delta F_p/\delta\mathbf{p}$. The Fokker-Planck equation can then be written as

$$\partial_t \Pi = \int_{\mathbf{x}} \nabla_{\mathbf{p}}\cdot[-(\nu\mathbf{m}\Pi) + \tilde{\Gamma}_p\{\mathbf{h} + D\nabla_{\mathbf{p}}\}\Pi] + \frac{1}{\tau_p}\nabla_{\mathbf{m}}\cdot\left(\mathbf{m} + \frac{D_m}{\tau_p}\nabla_{\mathbf{m}}\right)\Pi. \tag{S31}$$

As in the $\phi^4$ model, we would like to find $R_0[p_x, p_y] = \int dm_x dm_y \Pi$ to first order in $\tau_p$. For this, we define the moments $\mathbf{R}_{1i} = \int dm_x dm_y m_i \Pi$, $\mathbf{R}_{2ij} = \int dm_x dm_y m_i m_j \Pi$ and $\mathbf{R}_{3ijk} = \int dm_x dm_y m_i m_j m_k \Pi$. The equation of motion for these moments are (suppressing the overall integral)

$$\partial_t R_0 = \nabla_{\mathbf{p}}\cdot\left[-\nu\mathbf{R}_1 + \tilde{\Gamma}_p\{\mathbf{h} + D\nabla_{\mathbf{p}}\}R_0\right] \tag{S32}$$

$$\partial_t R_{1i} = \nabla_{p_j}\left[-\nu R_{2ij} + \tilde{\Gamma}_p\{h_j + D\nabla_{p_j}\}R_{1i}\right] - \frac{R_{1i}}{\tau_p} \tag{S33}$$

$$\partial_t R_{2ij} = \nabla_{p_k}\left[-\nu R_{3ijk} + \tilde{\Gamma}_p\{h_k + D\nabla_{p_k}\}R_{2ij}\right] - \frac{2R_{2ij}}{\tau_p} + \delta_{ij}\frac{2D_m}{\tau_p^2}R_0 \tag{S34}$$

$$\partial_t R_{3ijk} = \nabla_{p_l}\left[-\nu R_{4ijkl} + \tilde{\Gamma}_p\{h_l + D\nabla_{p_l}\}R_{3ijk}\right] - \frac{3R_{3ijk}}{\tau_p} + \frac{2D_m}{\tau_p^2}[R_{1i}\delta_{jk} + R_{1j}\delta_{ik} + R_{1k}\delta_{ij}] \tag{S35}$$

In the $\tau_p \to 0$ limit, in the steady state we obtain using (S34), (S33) and (S32) (in that order),

$$\mathbf{R}_1 = -\nu D_m \nabla_{\mathbf{p}} R_0 \implies \tilde{\Gamma}_p \nabla_{\mathbf{p}}\cdot\left[\mathbf{h} + \left(D + \frac{\nu^2 D_m}{\tilde{\Gamma}_p}\right)R_0\right] = 0 \implies R_0 \propto e^{-F_p/\tilde{D}} \tag{S36}$$

where $\tilde{D} = D + \nu^2 D_m/\tilde{\Gamma}_p$. To calculate the $\mathcal{O}(\tau_\phi)$ correction, we use (S35) to obtain

$$R_{3ijk} = \frac{2D_m}{3\tau_p}[R_{1i}\delta_{jk} + R_{1j}\delta_{ik} + R_{1k}\delta_{ij}] \tag{S37}$$

which yields

$$R_{2xx} = -\nu D_m\left[\partial_{p_x}R_{1x} + \frac{1}{3}\partial_{p_y}R_{1y}\right] + \frac{D_m}{\tau_p}R_0 \tag{S38}$$

$$R_{2xy} = -\frac{\nu D_m}{3}\left[\partial_{p_x} R_{1y} + \partial_{p_y} R_{1x}\right] \tag{S39}$$

$$R_{2yy} = -\nu D_m\left[\frac{1}{3}\partial_{p_x} R_{1x} + \partial_{p_y} R_{1y}\right] + \frac{D_m}{\tau_p} R_0 \tag{S40}$$

which in turn yields

$$\partial_{p_i} R_{1i} = -\nu D_m {\partial_{p_i}}^2 R_0 + \tau_p \nu^2 D_m \partial_{p_i} {\partial_{p_k}}^2 R_{1i} + \tau_p \partial_{p_i}\partial_{p_j}\left[\tilde{\Gamma}_p\{h_j + D\partial_{p_j}\} R_{1i}\right] = -\nu D_m {\partial_{p_i}}^2 R_0 + \tau_p \partial_{p_i}\partial_{p_j}\left[\tilde{\Gamma}_p\{h_j + \tilde{D}\partial_{p_j}\} R_{1i}\right] \tag{S41}$$

As in the $\phi^4$ model, we expand $R_0 = R_0^0 + \tau_p R_0^1$ and $\mathbf{R}_1 = \mathbf{R}_1^0 + \tau_p \mathbf{R}_1^1$ and note

$$R_{1i}^0 = \frac{\nu D_m}{\tilde{D}} \frac{\partial f_p}{\partial p_i} R_0^0 = \frac{\nu D_m}{\tilde{D}} h_i R_0^0 \tag{S42}$$

This then yields an equation for $R_0^1$:

$$[h_i + \tilde{D}\partial_{p_i}] R_0^1 = \nu \partial_{p_j}\left(h_j + \tilde{D}\partial_{p_j}\right) R_{1i}^0. \tag{S43}$$

Therefore,

$$\partial_{p_i}[e^{F_p/\tilde{D}} R_0^1] = \frac{\nu^2 D_m}{\tilde{D}} \partial_{p_i}\left[\tilde{D}{\partial_{p_j}}^2 f_p - \frac{1}{2}(\partial_{p_j} f_p)^2\right] \tag{S44}$$

This implies that

$$R_0 \propto e^{\tilde{F}_p/\tilde{D}};\; \tilde{F}_p = \int d\mathbf{x} \tilde{f}_p; \quad \tilde{f}_p = f_p + \frac{\nu^2 D_m \tau_p}{\tilde{D}}\left[\frac{1}{2}(\partial_{p_j} f_p)^2 - \tilde{D}{\partial_{p_j}}^2 f_p\right] \tag{S45}$$

where, as in the $\phi^4$ model, only terms explicitly depending on $\mathbf{p}$ are retained for the expression in the square brackets (terms independent of $\mathbf{p}$ are eliminated by the derivative of the R.H.S. of (S44)). Noting that $f_p$ only depends on the magnitude of $\mathbf{p}$, $p = |\mathbf{p}|$, we can reexpress the effective potential as

$$\tilde{f}_p = f_p + \frac{\nu^2 D_m \tau_p}{\tilde{D}}\left[\frac{1}{2}(\partial_p f_p)^2 - \tilde{D}\partial_p^2 f_p\right] \tag{S46}$$

Using $f_p$ from (S28),

$$\tilde{f}_p = \frac{1}{2}\left[\alpha + \frac{\nu^2 D_m \tau_p(\alpha^2 - 6\tilde{D}\beta)}{\tilde{D}}\right] p^2 + \frac{\beta}{4}\left(1 + \frac{4\nu^2 D_m \alpha \tau_p}{\tilde{D}}\right) p^2 + \frac{\nu^2 D_m \beta^2 \tau_p}{2\tilde{D}} p^6 \tag{S47}$$

This demonstrates that increasing the value of $\nu^2 D_m$ (which also leads to an increase in the value of $\tilde{D}$) leads to the coefficient of the $p^2$ term in $\tilde{f}_p$ changing sign signalling a mean-field transition to an ordered state. However, while polar ordered active phases on substrates are known to have long-range order even in two dimensions, this will not be case here. The field $\mathbf{m}$ does not order along with $\mathbf{p}$ since its dynamics is autonomous and $\mathbf{p}$ is not motile. Thus, the ordered phase to $\mathcal{O}(\tau_p)$ is effectively in equilibrium and immotile implying that it cannot escape the Mermin-Wagner theorem [3, 4]. More formally, polar active phases have long-range order due to self-advection $\sim \mathbf{p}\cdot\nabla\mathbf{p}$ but no such term can appear here and the term $\sim \mathbf{m}\cdot\nabla\mathbf{p}$ that does (due to the advective nonlinearity in $\mathbf{p}$) cannot lead to a wavevector dependent correction to the effective "diffusion" constant for the angular fluctuations. Therefore, the polar phase here will only have quasi-long-range order in two dimensions as in equilibrium systems.

## III. DETAILED CALCULATION FOR THE APOLAR MODEL

We now consider a system of rods immersed in a momentum conserving active fluid composed of active particles that exert dipolar forces but have no shape asymmetry. The standard model for the dynamics of the apolar order parameter

$$\mathbf{Q} = \begin{pmatrix} Q_{xx} & Q_{xy} \\ Q_{xy} & -Q_{xx} \end{pmatrix} \tag{S48}$$

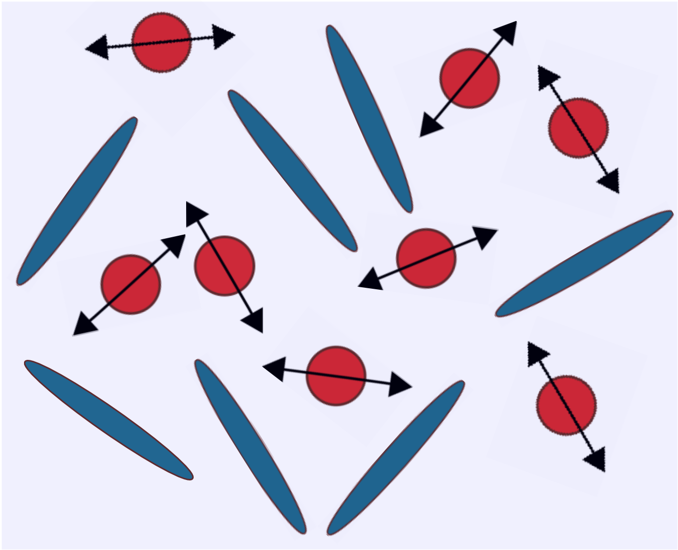

FIG. 1: Suspension of apolar rods, denoted by blue ellipsoids, in a momentum-conserving bath of isotropic active particles, denoted by red circles. The double arrow denotes the force dipole direction.

which is a symmetric, traceless tensor, in a fluid is

$$D_t\mathbf{Q} = \lambda\mathbf{A} - \Gamma\frac{\delta F}{\delta\mathbf{Q}} + \sqrt{2\Gamma D}\boldsymbol{\chi} \tag{S49}$$

where $D_t = \partial_t + \mathbf{v}\cdot + [\boldsymbol{\Omega}.]^A$ is the co-rotational and advected derivative, with $\boldsymbol{\Omega}$ being the antisymmetric velocity gradient and the final term implying an antisymmetric contraction with $\mathbf{Q}$, $\mathbf{A} = (\nabla\mathbf{v} + (\nabla\mathbf{v})^T)/2$, with the superscript $T$ denoting transposition, $\lambda$ is the usual flow-alignment parameter that implies that shearing a nematic fluid tends to order it along the shearing direction, $\Gamma$ is a dissipative kinetic coefficient and $\boldsymbol{\chi}$ is a Gaussian white noise of unit variance which would have led to the steady-state probability distribution $\propto e^{-F/D}$ if the model were passive. We assume the free energy to be$F = \int d\mathbf{x} f$, which we take to have the simple mean-field form

$$f = \frac{\alpha}{2}\mathbf{Q}:\mathbf{Q} + \frac{\beta}{4}(\mathbf{Q}:\mathbf{Q})^2. \tag{S50}$$

The constitutive equation for the fluid velocity, in the Stokes limit appropriate for slow flows, is

$$-\eta\nabla^2\mathbf{v} = -\nabla\Pi + \frac{\lambda}{2}\nabla\cdot\frac{\delta F}{\delta\mathbf{Q}} + \frac{\zeta}{2}\nabla\cdot\mathbf{M} + \sqrt{-2D\eta\nabla^2}\boldsymbol{\Xi}. \tag{S51}$$

Here, $\eta$ is the viscosity, $\Pi$ is a pressure that acts as a Lagrange multiplier to enforce the incompressibility constraint $\nabla\cdot\mathbf{v} = 0$ and $\boldsymbol{\Xi}$ is a unit variance Gaussian white noise. Onsager symmetry, which would be operational in the limit of vanishing activity dictates the presence of the force $\propto\lambda$ in the velocity equation. Finally, the velocity field is forced by an active stress $\mathbf{M}$ with the coefficient $\zeta$ which models the dipolar forcing due to the active particles. Since the isotropic part of $\mathbf{M}$ cannot affect the velocity field in this incompressible fluid, instead only renormalising the pressure, we can take $\mathbf{M}$ to be trace-free without loss of generality i.e. $\mathbf{M} = \begin{pmatrix} m_{xx} & m_{xy} \\ m_{xy} & -m_{xx}\end{pmatrix}$. The dynamics of $\mathbf{M}$ is not affected by flow since the active particles we consider are spherical and is simply

$$\tau\partial_t\mathbf{M} = -\mathbf{M} + \sqrt{2D_M}\boldsymbol{\xi} \tag{S52}$$

where $\boldsymbol{\xi}$ is a Gaussian white noise of unit variance and $\tau$ is the characteristic relaxation time of the active stress. Note that while the strength of the noises in (S49) and (S51) are both proportional to $D$, we take the strength of the noise in the relaxational dynamics of $\mathbf{M}$ to be distinct from $D$. Now, defining $\mathbf{H} = \delta F/\delta\mathbf{Q} = \partial f/\partial\mathbf{Q}$, we Fourier transform the dynamical equations to eliminate the velocity field and obtain

$$\partial_t Q^k_{xx} = -\left(\Gamma + \frac{\lambda^2 k_x^2 k_y^2}{\eta k^4}\right) H^k_{xx} - \frac{\lambda^2 k_x k_y (k_y^2 - k_x^2)}{2\eta k^4} H^k_{xy} - \frac{\lambda^2 k_x^2 k_y^2}{\eta k^4} M^k_{xx} - \frac{\lambda^2 k_x k_y (k_y^2 - k_x^2)}{2\eta k^4} M^k_{xy} + \chi^k_1 \tag{S53}$$

$$\partial_t Q^k_{xy} = -\left(\Gamma + \frac{\lambda^2 (k_y^2 - k_x^2)^2}{4\eta k^4}\right) H^k_{xy} - \frac{\lambda^2 k_x k_y (k_y^2 - k_x^2)}{2\eta k^4} H^k_{xx} - \frac{\lambda^2 (k_y^2 - k_x^2)^2}{4\eta k^4} M^k_{xy} - \frac{\lambda^2 k_x k_y (k_y^2 - k_x^2)}{2\eta k^4} M^k_{xx} + \chi^k_2 \tag{S54}$$

where the superscript $k$ denotes the Fourier index and the noise correlators are

$$\langle \chi_1^{\mathbf{k}} \chi_1^{\mathbf{k}'} \rangle = 2D\left(\Gamma + \frac{\lambda^2 k_x^2 k_y^2}{\eta k^4}\right)\delta(t-t')\delta(\mathbf{k}+\mathbf{k}') \tag{S55}$$

$$\langle \chi_2^{\mathbf{k}} \chi_2^{\mathbf{k}'} \rangle = 2D\left(\Gamma + \frac{\lambda^2 (k_y^2 - k_x^2)^2}{4\eta k^4}\right)\delta(t-t')\delta(\mathbf{k}+\mathbf{k}') \tag{S56}$$

$$\langle \chi_1^{\mathbf{k}} \chi_2^{\mathbf{k}'} \rangle = 2D\frac{\lambda^2 k_x k_y (k_y^2 - k_x^2)}{2\eta k^4}\delta(t-t')\delta(\mathbf{k}+\mathbf{k}') \tag{S57}$$

This yields the Fokker-Planck equation

$$\begin{aligned}\partial_t \Pi = \sum_{\mathbf{k}} \Bigg[ &\left(\Gamma + \frac{\lambda^2 k_x^2 k_y^2}{\eta k^4}\right)\partial_{Q^k_{xx}}(H^k_{xx} + D\partial_{Q^k_{xx}})\Pi + \frac{\lambda^2 k_x k_y (k_y^2 - k_x^2)}{2\eta k^4}\partial_{Q^k_{xx}}(H^k_{xy} + D\partial_{Q^k_{xy}})\Pi \\ &+ \frac{\lambda^2 k_x k_y (k_y^2 - k_x^2)}{2\eta k^4}\partial_{Q^k_{xy}}(H^k_{xx} + D\partial_{Q^k_{xx}})\Pi + \left(\Gamma + \frac{\lambda^2 (k_y^2 - k_x^2)^2}{4\eta k^4}\right)\partial_{Q^k_{xy}}(H^k_{xy} + D\partial_{Q^k_{xy}})\Pi + \\ &\frac{\lambda\zeta k_x^2 k_y^2}{\eta k^4})\partial_{Q^k_{xx}}(M^k_{xx}\Pi) + \frac{\lambda\zeta k_x k_y (k_y^2 - k_x^2)}{2\eta k^4}\partial_{Q^k_{xy}}(M^k_{xx}\Pi) + \frac{\lambda\zeta k_x k_y (k_y^2 - k_x^2)}{2\eta k^4}\partial_{Q^k_{xx}}(M^k_{xy}\Pi) + \frac{\lambda\zeta (k_y^2 - k_x^2)^2}{4\eta k^4}\partial_{Q^k_{xy}}(M^k_{xy}\Pi) \\ &+ \frac{1}{\tau}\partial_{M^k_{xx}}\left(M^k_{xx} + \frac{D_M}{\tau}\partial_{M^k_{xx}}\right)\Pi + \frac{1}{\tau}\partial_{M^k_{xy}}\left(M^k_{xy} + \frac{D_M}{\tau}\partial_{M^k_{xy}}\right)\Pi\Bigg]\end{aligned} \tag{S58}$$

Since we are in the isotropic phase, the distribution function should be isotropic. Therefore, we write $\mathbf{k} = k_x\hat{x} + k_y\hat{y} = k(\cos\phi\hat{x} + \sin\phi\hat{y})$ and average (S58) over $\phi$ to obtain

$$\begin{aligned}\partial_t \Pi = \sum_{k} \Bigg[ &\tilde{\Gamma}\{\partial_{Q^k_{xx}}(H^k_{xx} + D\partial_{Q^k_{xx}})\Pi + \partial_{Q^k_{xy}}(H^k_{xy} + D\partial_{Q^k_{xy}})\Pi\} + \tilde{\zeta}\{\partial_{Q^k_{xx}}(M^k_{xx}\Pi) + \partial_{Q^k_{xy}}(M^k_{xy}\Pi)\} \\ &+ \frac{1}{\tau}\partial_{M^k_{xx}}\left(M^k_{xx} + \frac{D_M}{\tau}\partial_{M^k_{xx}}\right)\Pi + \frac{1}{\tau}\partial_{M^k_{xy}}\left(M^k_{xy} + \frac{D_M}{\tau}\partial_{M^k_{xy}}\right)\Pi\Bigg]\end{aligned} \tag{S59}$$

where $\tilde{\Gamma} = \Gamma + \lambda^2/8\eta$ and $\tilde{\zeta} = \lambda\zeta/8\eta$. This implies that for $\tau \to 0$, one obtains the distribution function for $\mathbf{Q}$ marginalised over $M_{xx}$ and $M_{yy}$, $R_0 = \int dM_{xx}dM_{xy}\Pi$ as $e^{-F/\tilde{D}}$ where $\tilde{D} = D + \tilde{\zeta}^2 D_M/\tilde{\Gamma}$. To first order in $\tau$, following a procedure that parallels the one for the polar model, albeit now in the Fourier space , and finally Fourier transforming back to real space, we obtain

$$R_0 \propto e^{-\tilde{F}/\tilde{D}}; \quad \tilde{F} = \int d\mathbf{x}\tilde{f}; \quad \tilde{f} = f + \tau\frac{\tilde{\zeta}^2 D_M}{\tilde{D}}\left[\frac{1}{2}\left(\partial_{Q_{xx}}f^2 + \partial_{Q_{xy}}f^2\right) - \tilde{D}(\partial^2_{Q_{xx}} + \partial^2_{Q_{xy}})f\right] \tag{S60}$$

Just as in the polar model, the free energy depends merely on the magnitude of the order parameter $S = \sqrt{Q_{xx}^2 + Q_{xy}^2}$. Therefore, writing $f = \alpha S^2 + \beta S^4$, we can obtain an equivalent expression for the effective free energy as

$$\tilde{f} = f + \tau\frac{\tilde{\zeta}^2 D_M}{\tilde{D}}\left[\frac{1}{2}\left(\frac{\partial f}{\partial S}\right)^2 - \tilde{D}\frac{\partial^2 f}{\partial S^2}\right] \tag{S61}$$

Thus, the effective free energy as a function of $S$ becomes

$$\tilde{f}[S] = \left(\alpha + \frac{2\tilde{\zeta}^2 D_M \tau(\alpha^2 - 6\tilde{D}\beta)}{\tilde{D}}\right) S^2 + \left(\beta + \frac{8\tilde{\zeta}^2 D_M \alpha\beta\tau}{\tilde{D}}\right) S^4 + \frac{4\tilde{\zeta}^2 D_M \beta^2 \tau}{\tilde{D}} S^6 \tag{S62}$$

This demonstrates that the disordered phase of a system of rods in an active fluid can be rendered unstable at an arbitrarily high value of $\alpha$, and not only for $\alpha < 0$ (which since it may be controlled by the density of the apolar rods, means at arbitrarily low densities) by strong driving. For

$$D_M \tilde{\zeta}^2 > \frac{\alpha + 2\alpha^2\tilde{\Gamma}\tau - 12D\beta\tilde{\Gamma}\tau + \sqrt{48D\alpha\beta\tilde{\Gamma}\tau + (\alpha + 2\alpha^2\tilde{\Gamma}\tau - 12D\beta\tilde{\Gamma}\tau)^2}}{24\beta\tau} \tag{S63}$$

the coefficient of the $S^2$ term in $\tilde{f}$ turns negative signalling the destruction of the disordered phase. Since the active coupling does not destroy the ordered phase, an apolar phase may set in beyond this. This conclusion that increased active driving may lead to order may seem counter-intuitive. However, our calculation demonstrates that the finite correlation time of the active field is responsible for a generic upward shift of the mean-field critical point.

## IV. UNIFIED COLOURED NOISE APPROXIMATION FOR $\phi^4$ THEORY

In this appendix, we demonstrate that performing a unified coloured noise approximation (UCNA) [1] on a $\phi^4$ theory driven purely by a coloured noise leads to an effective probability distribution that is equivalent to (S18) in the limit in which $D = 0$. The dynamical equation we now consider is

$$\partial_t \phi(\mathbf{x}, t) = -\frac{\delta F_\phi}{\delta\phi(\mathbf{x})} + \xi_c(\mathbf{x}, t) \tag{S64}$$

where $F_\phi$ is given by (S2) and $\xi_c$ is a coloured noise given by

$$\tau_\phi \partial_t \xi_c = -\xi_c + \zeta \tag{S65}$$

with $\langle\zeta(\mathbf{x}, t)\zeta(\mathbf{x}', t')\rangle = 2D_\phi\delta(\mathbf{x}-\mathbf{x}')\delta(t-t')$. As is usual in UCNA, we take another derivative in (S64) and eliminate $\xi_c$ to obtain

$$\tau_\phi \partial_t^2 \phi(\mathbf{x}, t) = -\tau_\phi \int d\mathbf{x}' \frac{\delta^2 F_\phi}{\delta\phi(\mathbf{x})\delta\phi(\mathbf{x}')} \partial_t\phi(\mathbf{x}', t) + \tau_\phi\partial_t\xi_c = -\int d\mathbf{x}' \left[\delta(\mathbf{x}-\mathbf{x}') + \tau_\phi \frac{\delta^2 F_\phi}{\delta\phi(\mathbf{x})\delta\phi(\mathbf{x}')}\right] \partial_t\phi(\mathbf{x}', t) - \frac{\delta F_\phi}{\delta\phi(\mathbf{x})} + \zeta \tag{S66}$$

Ignoring the double time derivative on the R.H.S. in the spirit of U.C.N.A, this, to first order in $\tau_\phi$, becomes

$$\partial_t\phi(\mathbf{x}, t) = -\int d\mathbf{x}' \left[\delta(\mathbf{x}-\mathbf{x}') - \tau_\phi \frac{\delta^2 F_\phi}{\delta\phi(\mathbf{x})\delta\phi(\mathbf{x}')}\right] \frac{\delta F_\phi}{\delta\phi(\mathbf{x}')} + \int d\mathbf{x}' \left[\delta(\mathbf{x}-\mathbf{x}') - \tau_\phi \frac{\delta^2 F_\phi}{\delta\phi(\mathbf{x})\delta\phi(\mathbf{x}')}\right] \zeta(\mathbf{x}', t) \tag{S67}$$

The noise correlation is

$$\langle\nu(\mathbf{x}, t)\nu(\mathbf{x}', t')\rangle = \left\langle \int d\mathbf{x}'' d\mathbf{x}''' \left[\delta(\mathbf{x}-\mathbf{x}'') - \tau_\phi \frac{\delta^2 F_\phi}{\delta\phi(\mathbf{x})\delta\phi(\mathbf{x}'')}\right] \zeta(\mathbf{x}'', t) \left[\delta(\mathbf{x}'-\mathbf{x}''') - \tau_\phi \frac{\delta^2 F_\phi}{\delta\phi(\mathbf{x}')\delta\phi(\mathbf{x}''')}\right] \zeta(\mathbf{x}''', t) \right\rangle \tag{S68}$$

To first order in $\tau_\phi$, this yields

$$\langle\nu(\mathbf{x}, t)\nu(\mathbf{x}', t')\rangle = 2D_\phi\delta(t-t') \left[\delta(\mathbf{x}-\mathbf{x}') - 2\tau_\phi \frac{\delta^2 F_\phi}{\delta\phi(\mathbf{x})\delta\phi(\mathbf{x}')}\right] \tag{S69}$$

We can now write the Fokker-Planck equation corresponding to (S67) as

$$\begin{aligned}\partial_t\Pi[\phi(\mathbf{x})] = \int d\mathbf{x} \frac{\delta}{\delta\phi(\mathbf{x})} \Bigg[\Bigg\{ \int d\mathbf{x}' \left(\delta(\mathbf{x}-\mathbf{x}') - \tau_\phi \frac{\delta^2 F_\phi}{\delta\phi(\mathbf{x})\delta\phi(\mathbf{x}')}\right) \frac{\delta F_\phi}{\delta\phi(\mathbf{x}')} \\ - D_\phi \int d\mathbf{x}' \int d\mathbf{x}'' \left(\delta(\mathbf{x}-\mathbf{x}') - \tau_\phi \frac{\delta^2 F_\phi}{\delta\phi(\mathbf{x})\delta\phi(\mathbf{x}')}\right) \frac{\delta}{\delta\phi(\mathbf{x}')} \left(\delta(\mathbf{x}-\mathbf{x}'') - \tau_\phi \frac{\delta^2 F_\phi}{\delta\phi(\mathbf{x})\delta\phi(\mathbf{x}'')}\right) \Bigg\}\Pi[\phi(\mathbf{x})] \\ + D_\phi \int d\mathbf{x}') \frac{\delta}{\delta\phi(\mathbf{x}')} \left\{ \left(\delta(\mathbf{x}-\mathbf{x}') - 2\tau_\phi \frac{\delta^2 F_\phi}{\delta\phi(\mathbf{x})\delta\phi(\mathbf{x}')}\right) \Pi[\phi(\mathbf{x})] \right\} \Bigg]\end{aligned} \tag{S70}$$

To first order in $\tau_\phi$, this is equivalent to

$$\partial_t \Pi[\phi(\mathbf{x})] = \int d\mathbf{x} \frac{\delta}{\delta\phi(\mathbf{x})} \left[ \int d\mathbf{x}' \left( \delta(\mathbf{x}-\mathbf{x}') - 2\tau_\phi \frac{\delta^2 F_\phi}{\delta\phi(\mathbf{x})\delta\phi(\mathbf{x}')} \right) \left[ \left\{ \left( \delta(\mathbf{x}-\mathbf{x}') + \tau_\phi \frac{\delta^2 F_\phi}{\delta\phi(\mathbf{x})\delta\phi(\mathbf{x}')} \right) \frac{\delta F_\phi}{\delta\phi(\mathbf{x}')} - D_\phi \tau_\phi \frac{\delta}{\delta\phi(\mathbf{x}')} \frac{\delta^2 F_\phi}{\delta\phi(\mathbf{x})\delta\phi(\mathbf{x}')} \right\} \Pi[\phi(\mathbf{x})] + D_\phi \frac{\delta \Pi[\phi(\mathbf{x})]}{\delta\phi(\mathbf{x}')} \right] \right] \quad \text{(S71)}$$

We now take $\Pi \propto e^{-\tilde{F}_\phi/D_\phi}$. With this identification the term within the inner square brackets can be rewritten as

$$\frac{\delta}{\delta\phi(\mathbf{x}')} \left[ F_\phi + \frac{\tau_\phi}{2} \left( \frac{\delta F_\phi}{\delta\phi(\mathbf{x})} \right)^2 - D_\phi \tau_\phi \frac{\delta^2 F_\phi}{\delta\phi(\mathbf{x})\delta\phi(\mathbf{x}')} - \tilde{F}_\phi \right] e^{-\tilde{F}_\phi/D_\phi} \quad \text{(S72)}$$

The functional derivative is going to kill every term not explicitly dependent on $\phi$. Then, using the definition of $F_\phi$, a steady-state solution of the Fokker-Planck equation with zero current can be constructed as

$$\tilde{F}_\phi = \frac{1}{2} \int d\mathbf{x} \left[ \{\alpha + \tau_\phi(\alpha^2 - 6D_\phi\beta)\}\phi^2 + \beta \left( \frac{1 + 4\tau_\phi\alpha}{2} \right) \phi^4 + K(1 + 2\tau_\phi\alpha)(\nabla\phi)^2 + \tau_\phi\beta^2\phi^6 + \tau_\phi K(\nabla^2\phi)^2 + 6\tau_\phi\beta K\phi^2(\nabla\phi)^2 \right] \quad \text{(S73)}$$

As expected, this become equivalent to (S18) when we take the limit $D \to 0$ in that equation i.e., when we ignore the equilibrium white noise of the $\phi^4$ theory and only retain a coloured noise

---

* nyomaitra07@gmail.com

[1] P. Hänggi, P. Jung, Adv. Chem. Phys. **89**, 239 (1995); P Jung, P Hänggi, Phys. Rev. A **35**, 4464 (1987)
[2] Y Baek et al., Phys. Rev. Lett. **120**, 058002 (2018)
[3] J. Toner, Phys. Rev. E **86**, 031918 (2013)
[4] J. Toner, Y. Tu, Phys. Rev. E **58**, 4828 (1998)
